# Supplementary material for: Two-Photon Interference of Photons from Remote Tin-Vacancy Centers in Diamond
Source: arXiv:2412.17539 source file (2025-03-12)
Supplement: Supplementary file 1 [file 5_supplementary.tex]

To better understand this behaviour one can write the total wavefunction after the output port:
\begin{equation}
    |\psi\rangle_{34} = \frac{1}{\sqrt{2}} \left( |H, \omega_{II}\rangle |H, \omega_{I}\rangle - |V, \omega_{I}\rangle |V, \omega_{II}\rangle \right)
\end{equation}
To focus on the temporal characteristics of the photons, we decompose the two-photon state into spatio-temporal modes, 
representing the photon wavepackets with time-dependent functions \( \varPhi_I(t) \) and \( \varPhi_{II}(t) \), 
rather than an infinite set of frequency modes. This approach leads us to express the two-photon state in the spatio-temporal integrated form:

\begin{align}
    |\psi\rangle_{34} &= \frac{1}{\sqrt{2}} \int dt_3 \, dt_4 
    \left[ |H, \varPhi_{II}(t_3)\rangle |H, \varPhi_I(t_4)\rangle \right. \nonumber \\
    &\quad \left. - |V, \varPhi_I(t_3)\rangle |V, \varPhi_{II}(t_4)\rangle \right] = \\
    &\quad \frac{1}{\sqrt{2}} \int dt_3 \, dt_4 \varPhi(t_3) \varPhi(t_4)
    \left[ |H, t_3\rangle |H, t_4\rangle \right. \nonumber \\
    &\quad \left. - e^{i (\omega_I - \omega_{II})(t_3 - t_4)}
    |V, t_3\rangle |V, t_4\rangle \right] = \\
    &\quad \frac{1}{\sqrt{2}} \left[ |H, t_3\rangle |H, t_4\rangle \right. \nonumber \left. - e^{i (\omega_I - \omega_{II})(t_3 - t_4)}|V, t_3\rangle |V, t_4\rangle \right] 
  \end{align}

Assuming the emiters have similar linewidths the $\varPhi_I(t) \approx \varPhi_{II}(t)$, $\int_{-\infty}^{\infty} dt \, \varPhi^*(t) \varPhi(t) = 1$ and 
accounting for the phase difference between the photon detection events acquired with unitary evolution.

This means, that the "difference is erased" because the detector is no longer sensitive to the frequency difference within that time bin.
